# Supplementary material for: Nonparametric estimation of simplified vine copula models: comparison of methods
Source: arXiv:1701.00845 source file (2017-04-05)
Supplement: Supplementary file 1 [file appendix.tex]

\newpage
\appendix

\section{Results for alternative accuracy measures}

\begin{figure}
\centering
\includegraphics[width = \textwidth]{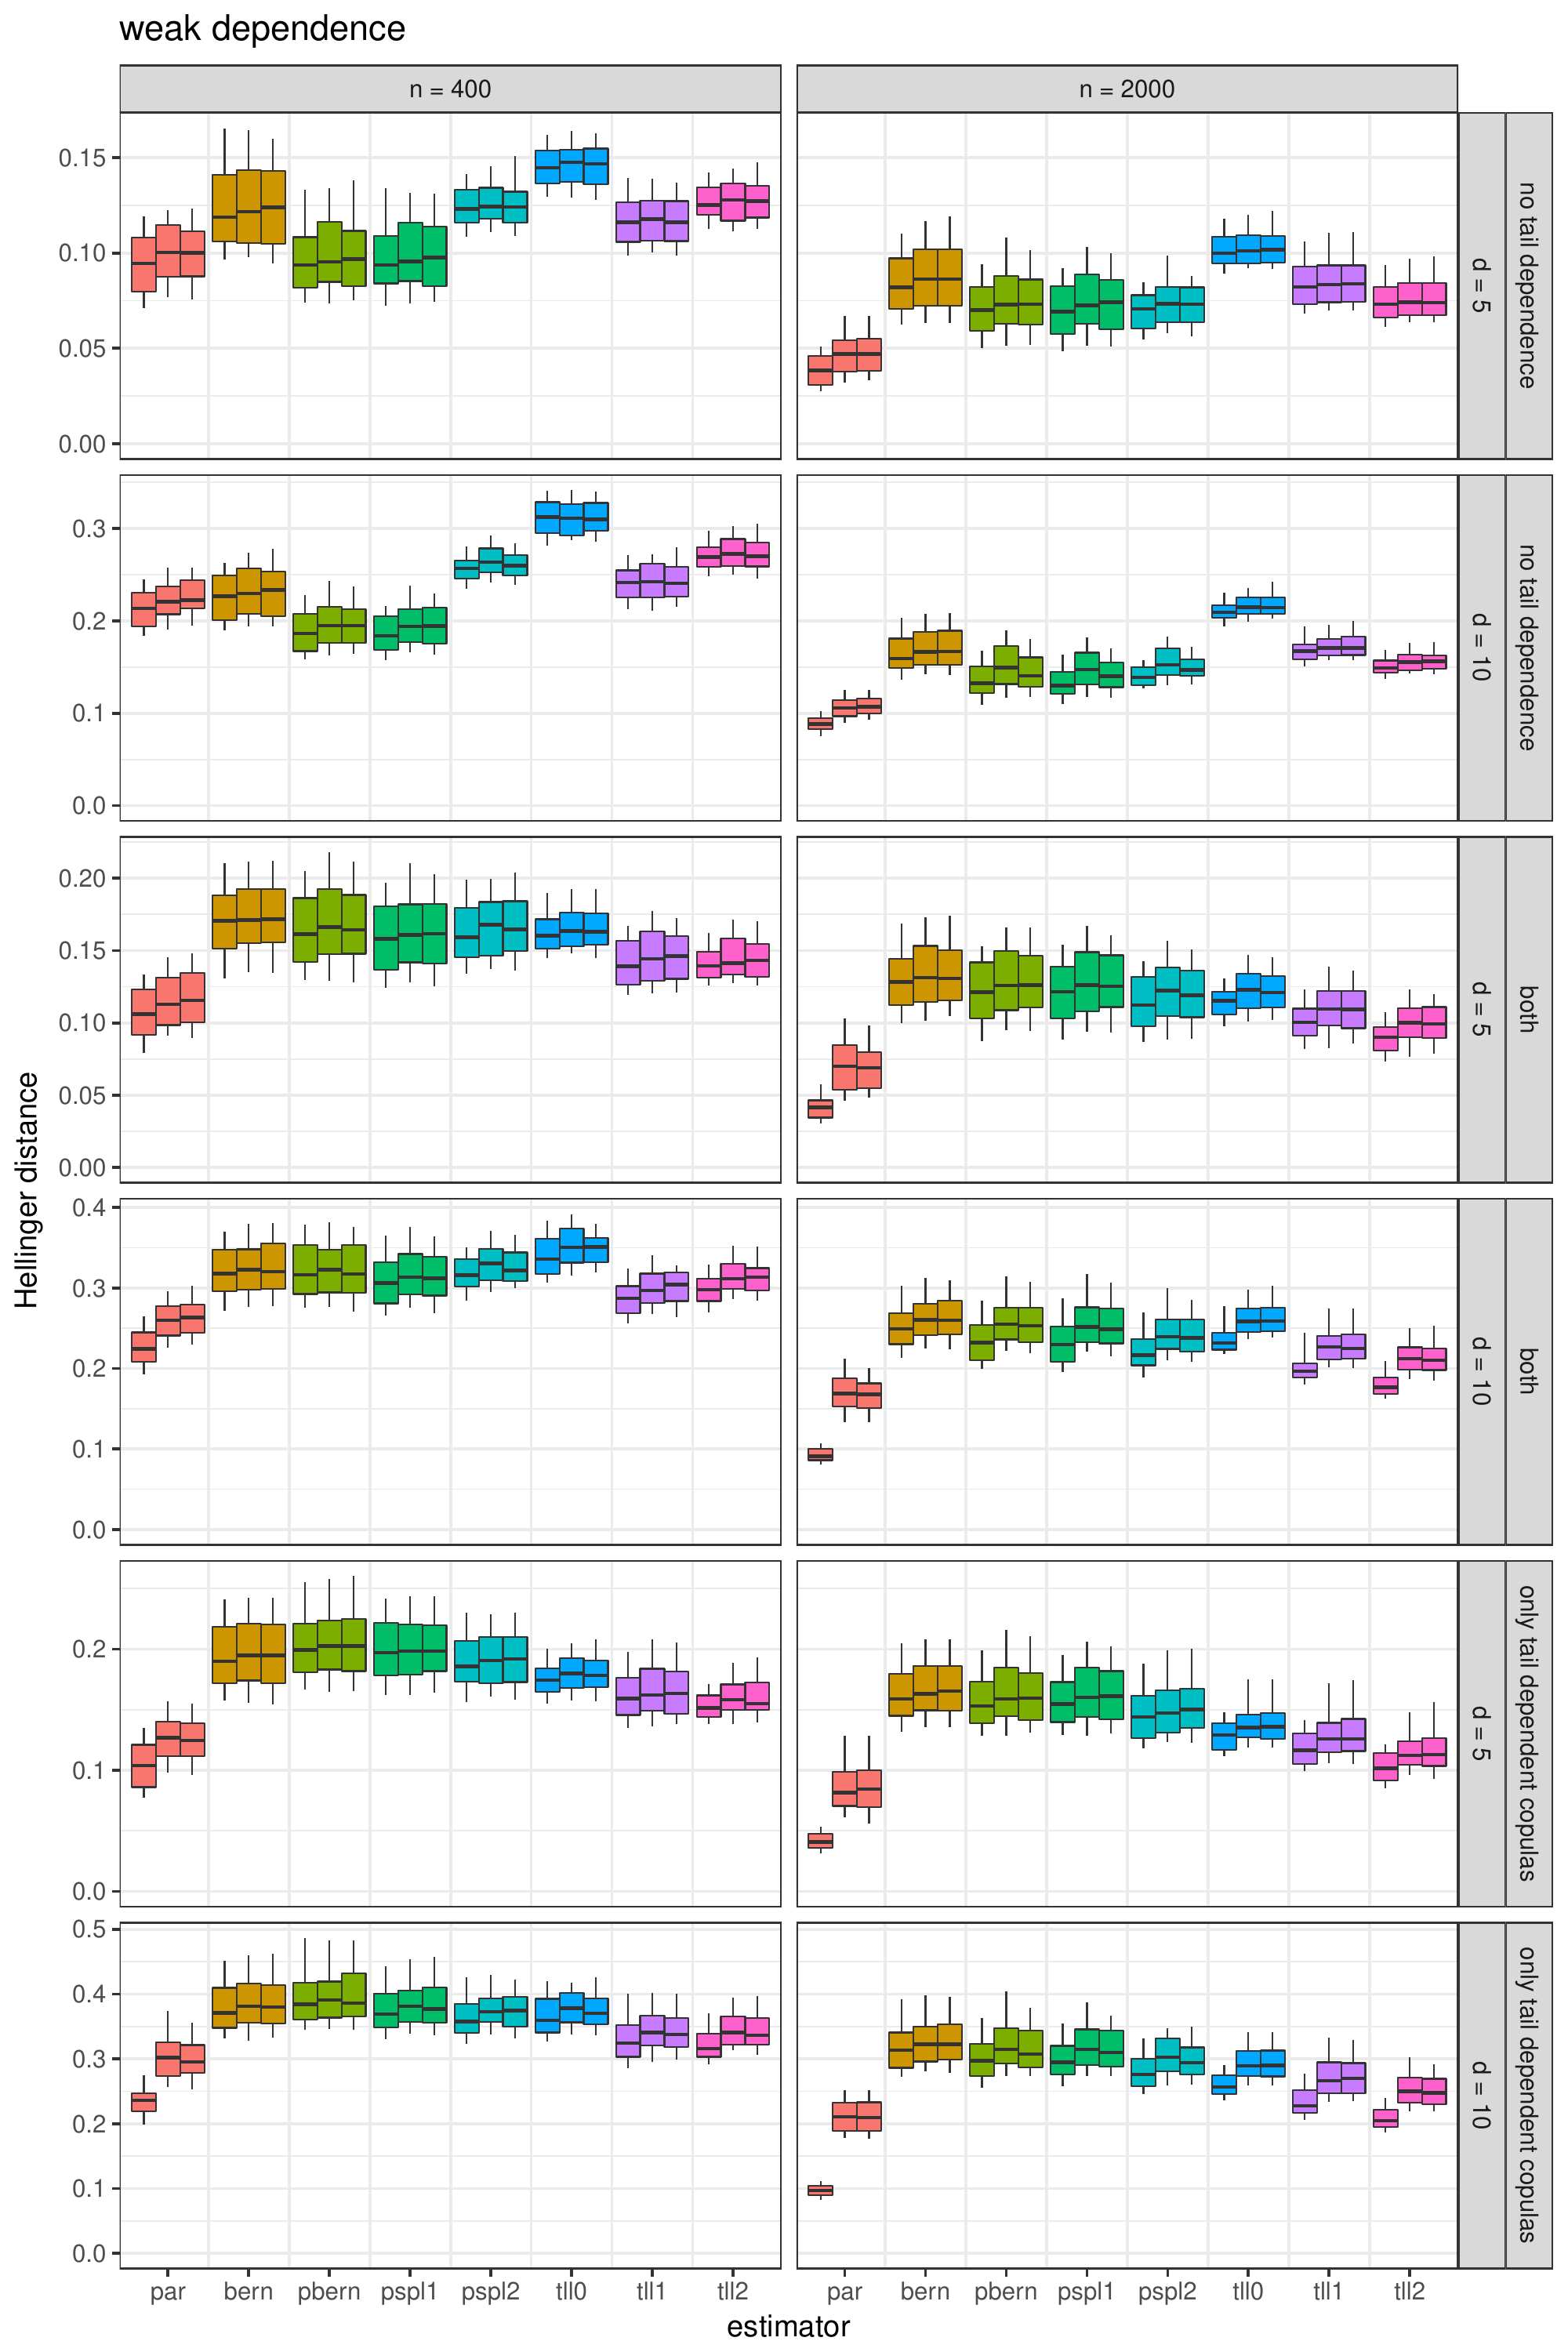}
\caption{\emph{weak dependence:} the box plots show the Hellinger distance achieved by each estimation method. Results are split by sample size, dimension, and type of dependence. Per estimator there are three boxes, corresponding to estimation under known structure, selection by Kendall's $\tau$, and selection by cAIC (from left to right).}
\end{figure}

\begin{figure}
\centering
\includegraphics[width = \textwidth]{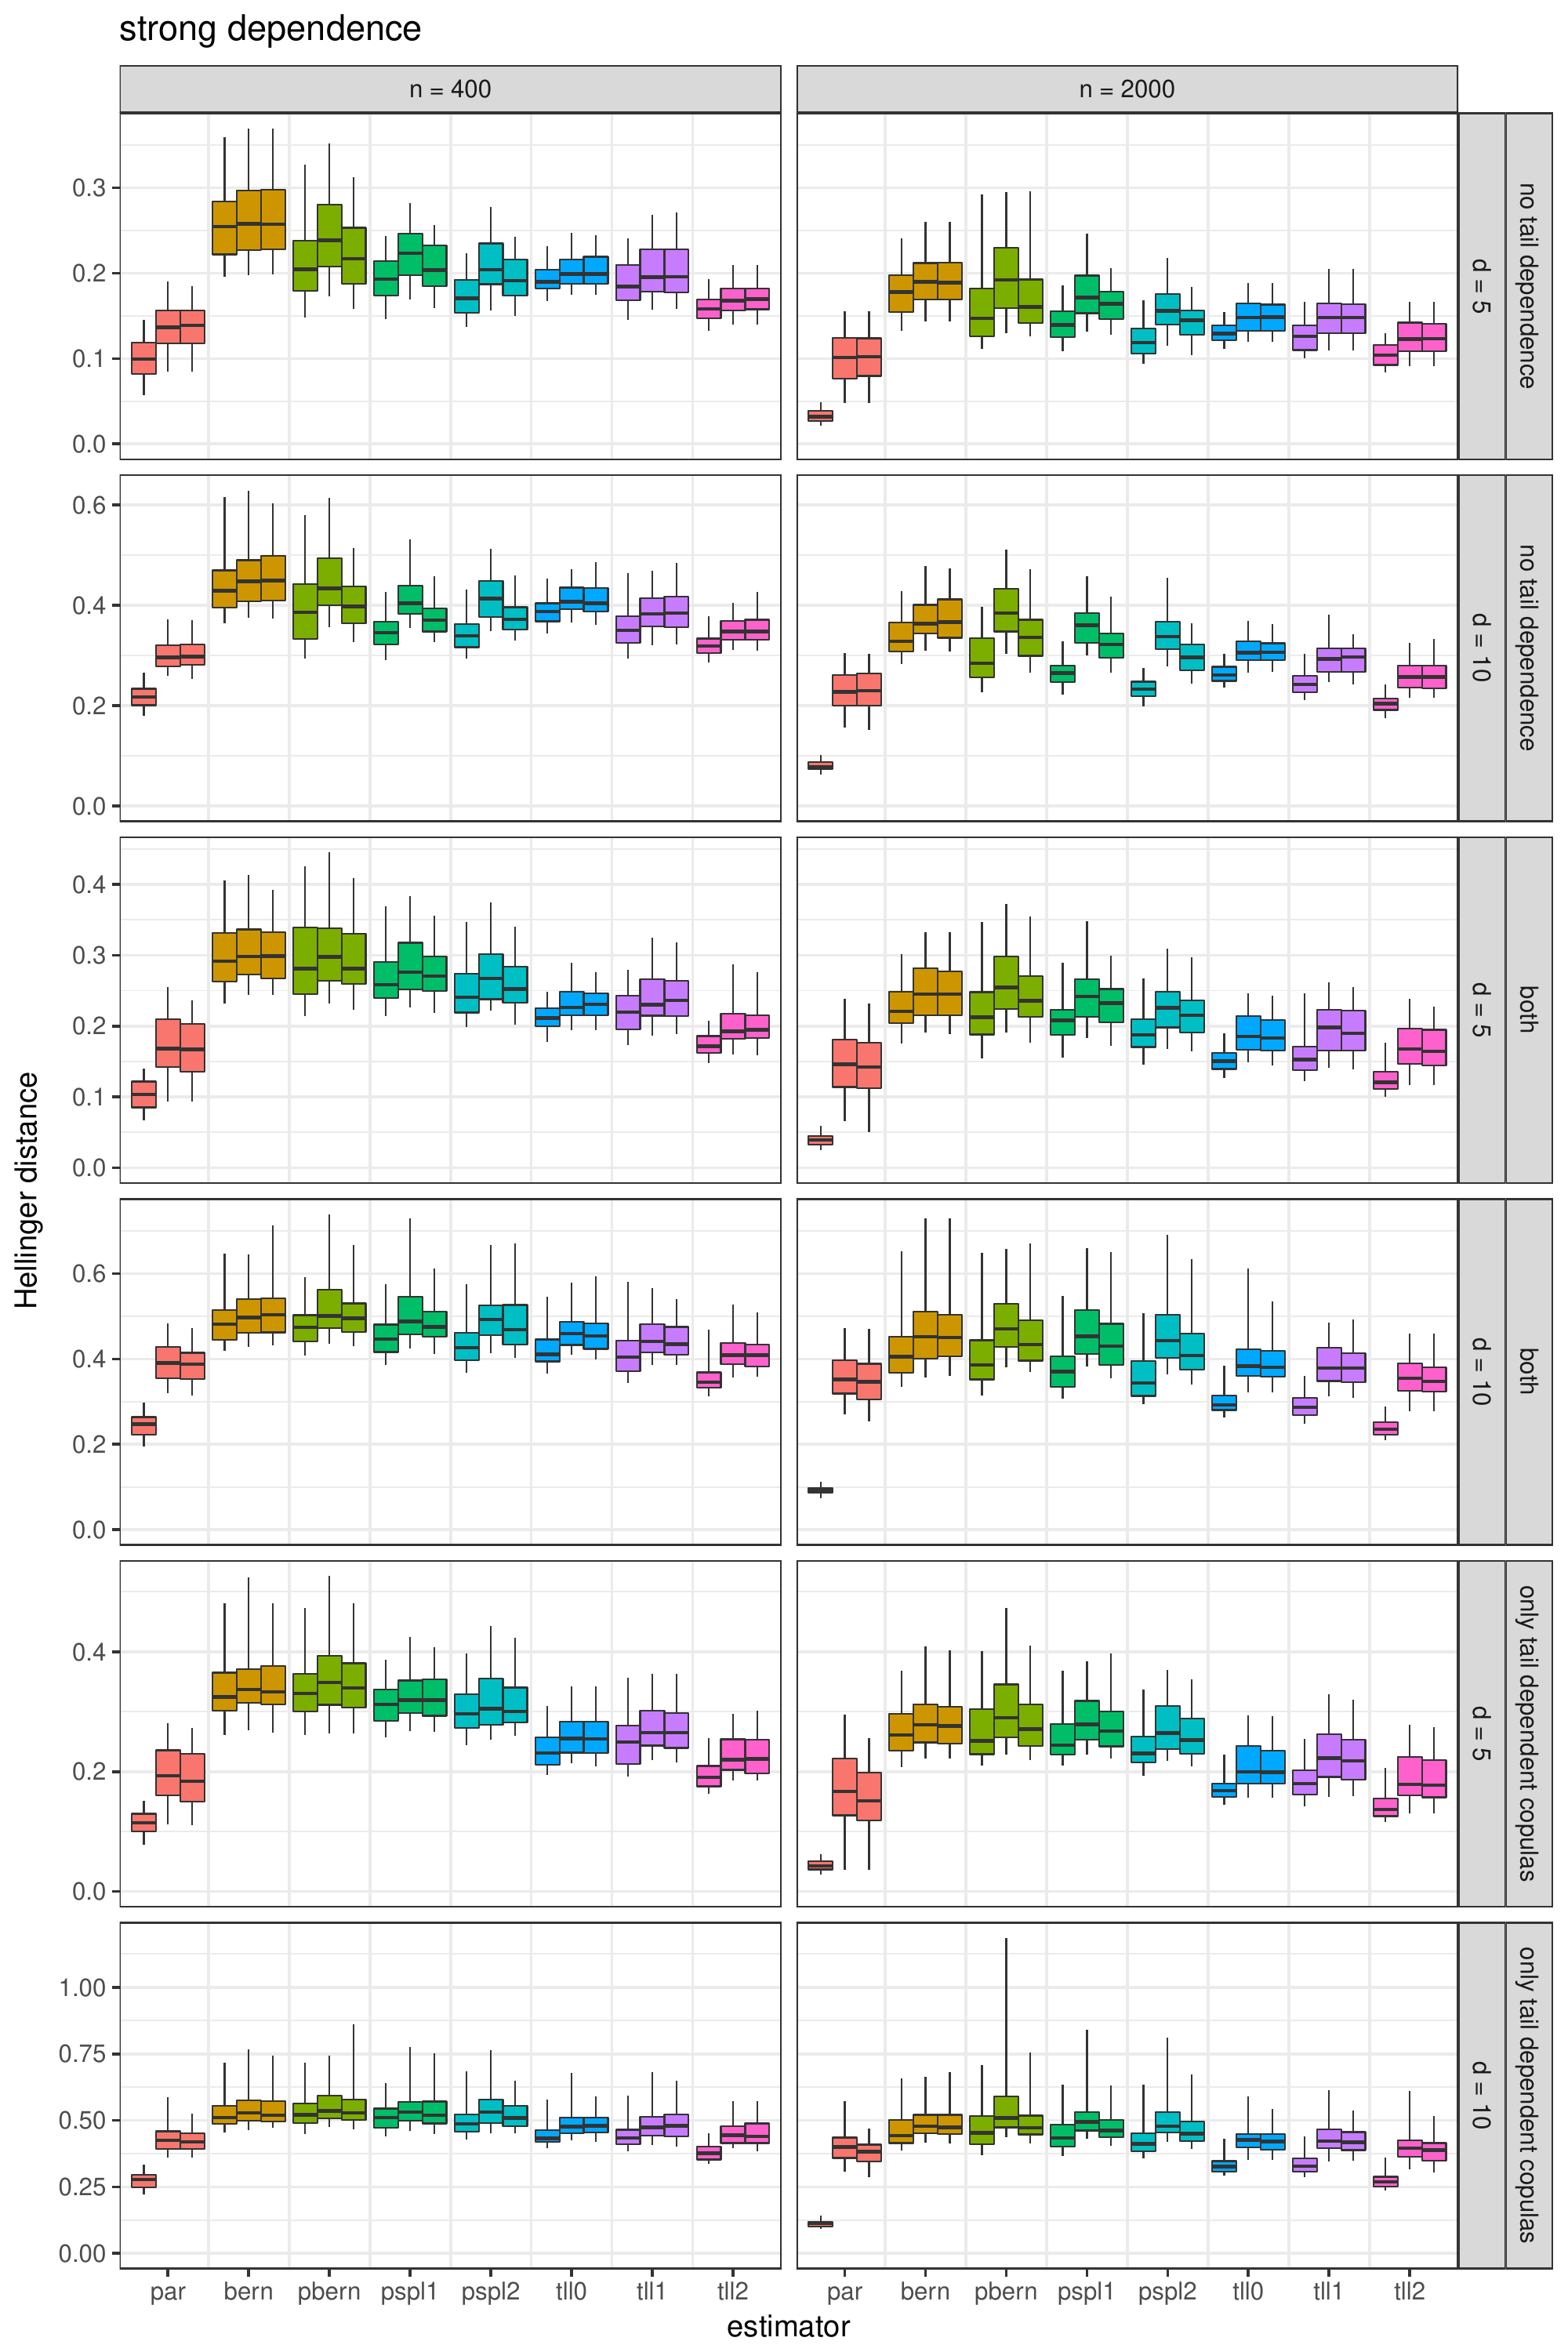} 
\caption{\emph{strong dependence:} the box plots show the Hellinger distance achieved by each estimation method. Results are split by sample size, dimension, and type of dependence.  Per estimator there are three boxes, corresponding to estimation under known structure, selection by Kendall's $\tau$, and selection by cAIC (from left to right).}
\end{figure}

\begin{figure}
\centering
\includegraphics[width = \textwidth]{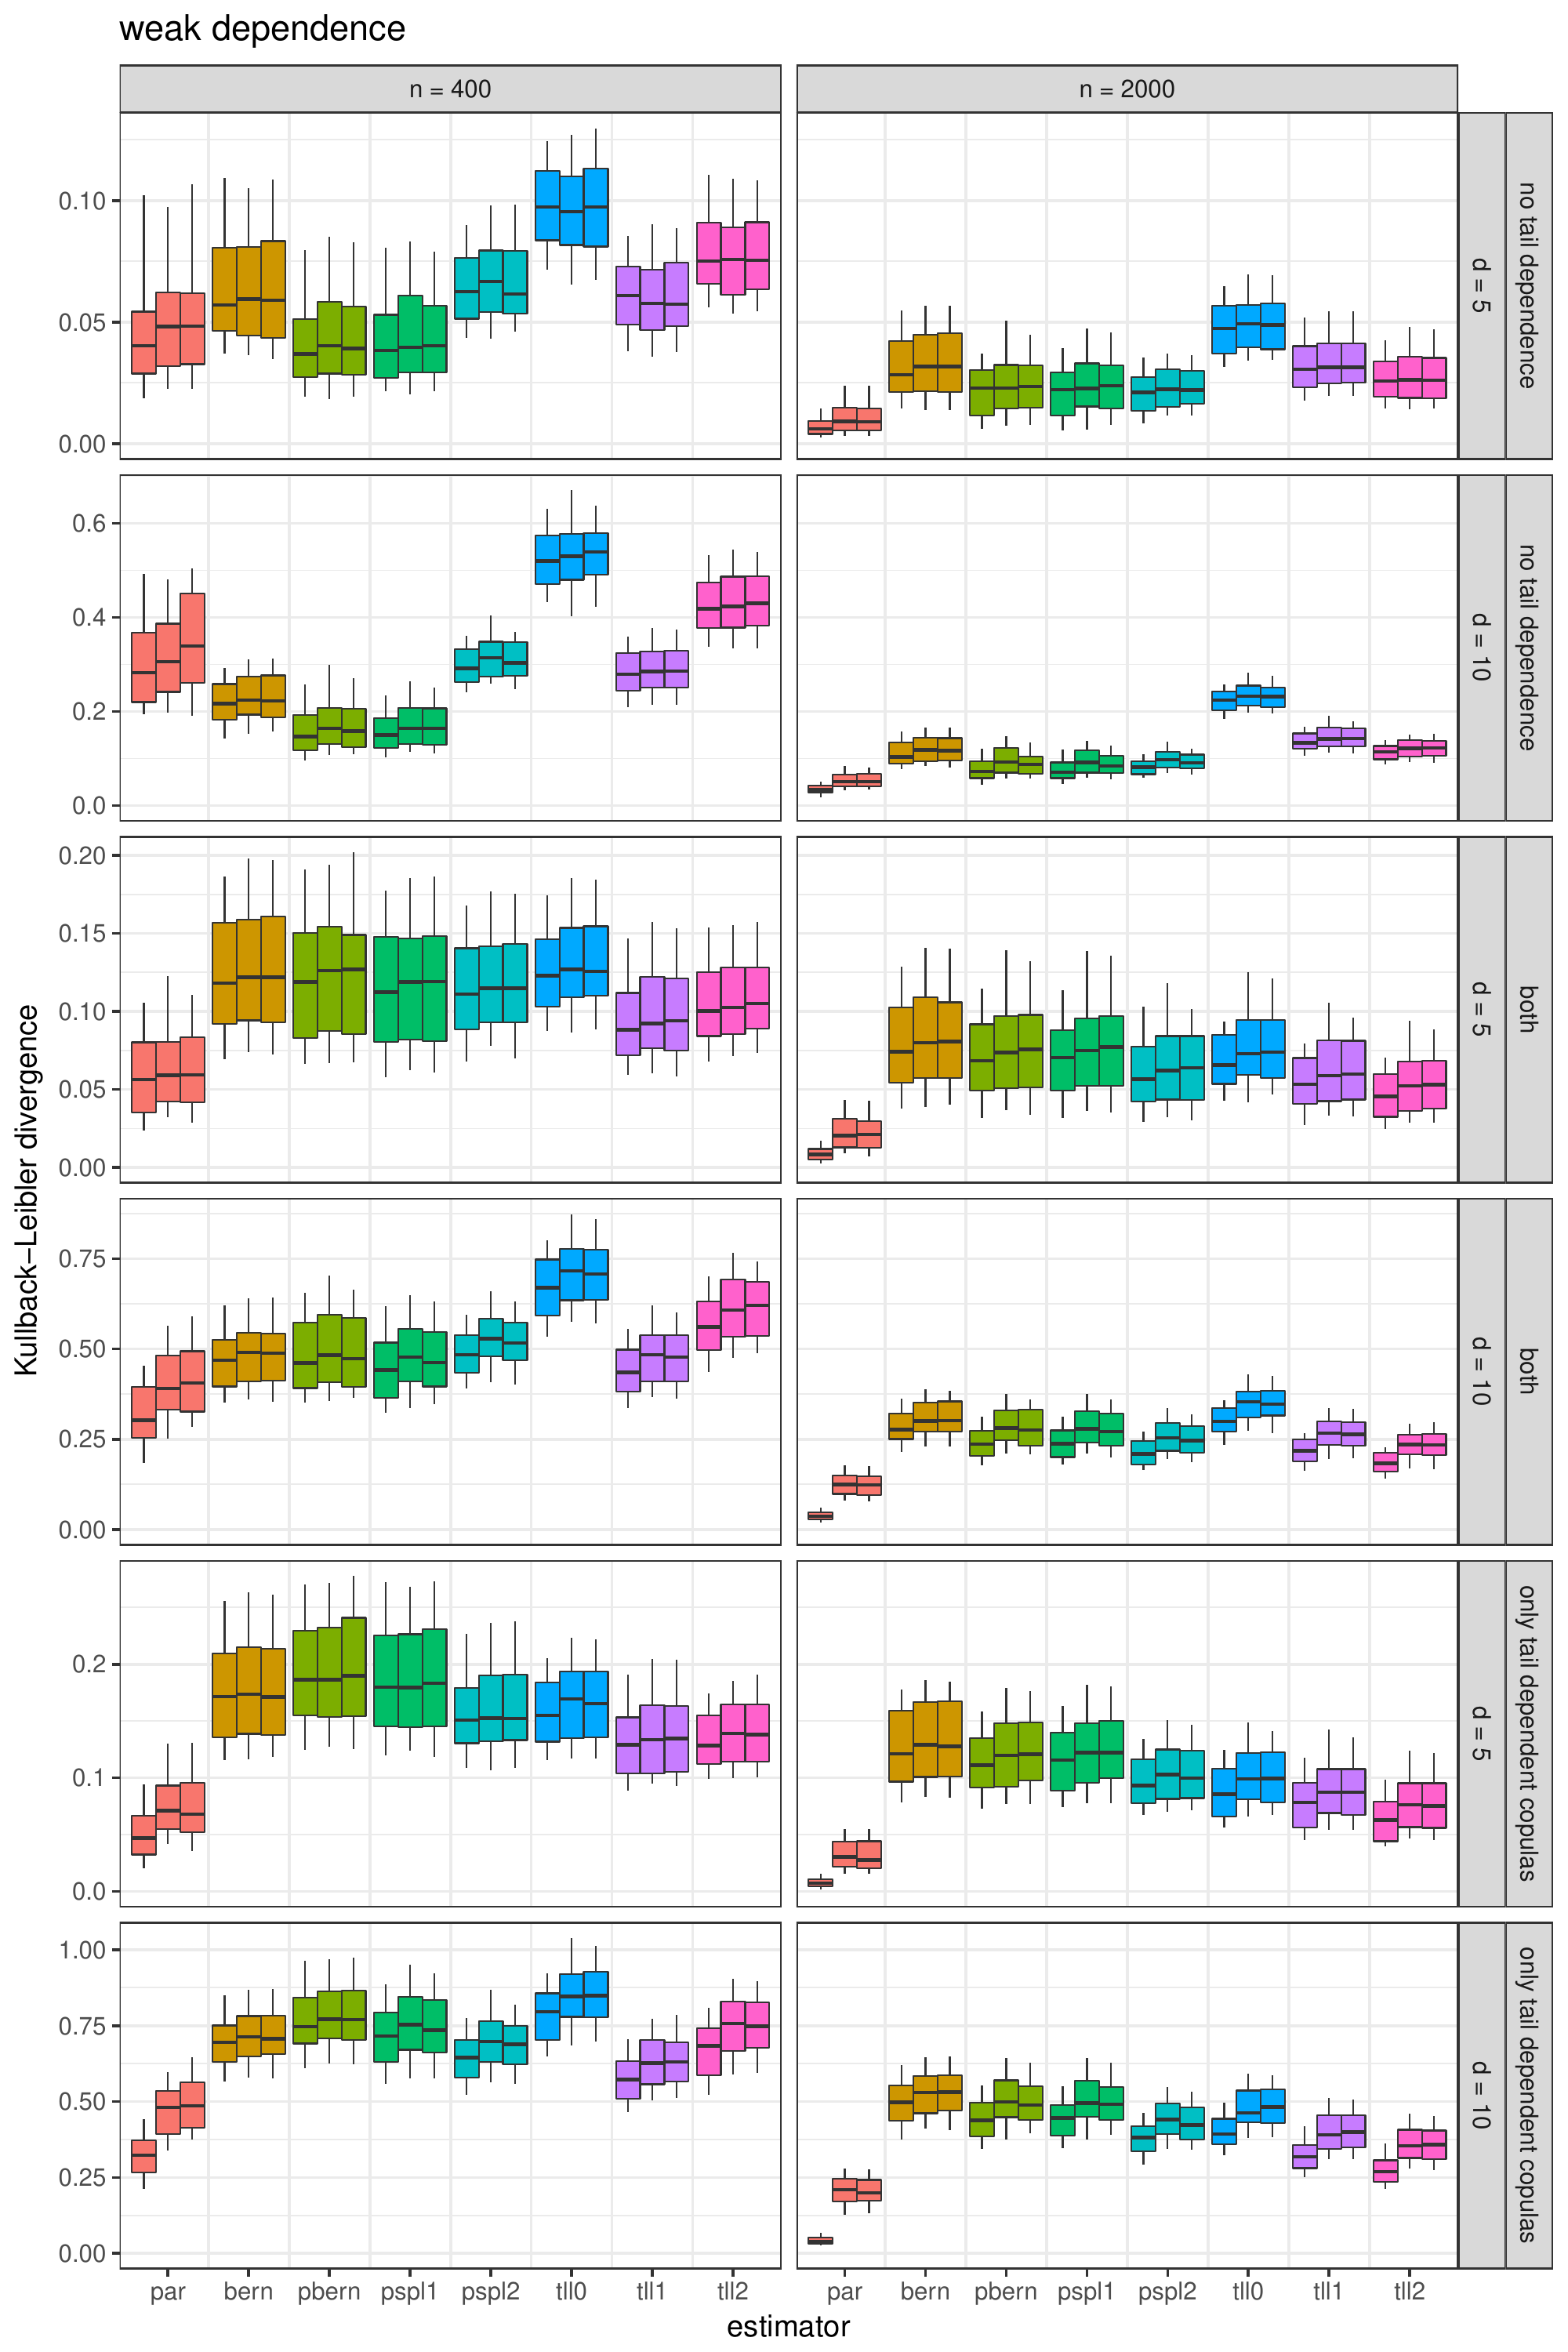}
\caption{\emph{weak dependence:} the box plots show the Kullback-Leibler divergence achieved by each estimation method. Results are split by sample size, dimension, and type of dependence. Per estimator there are three boxes, corresponding to estimation under known structure, selection by Kendall's $\tau$, and selection by cAIC (from left to right).}
\end{figure}

\begin{figure}
\centering
\includegraphics[width = \textwidth]{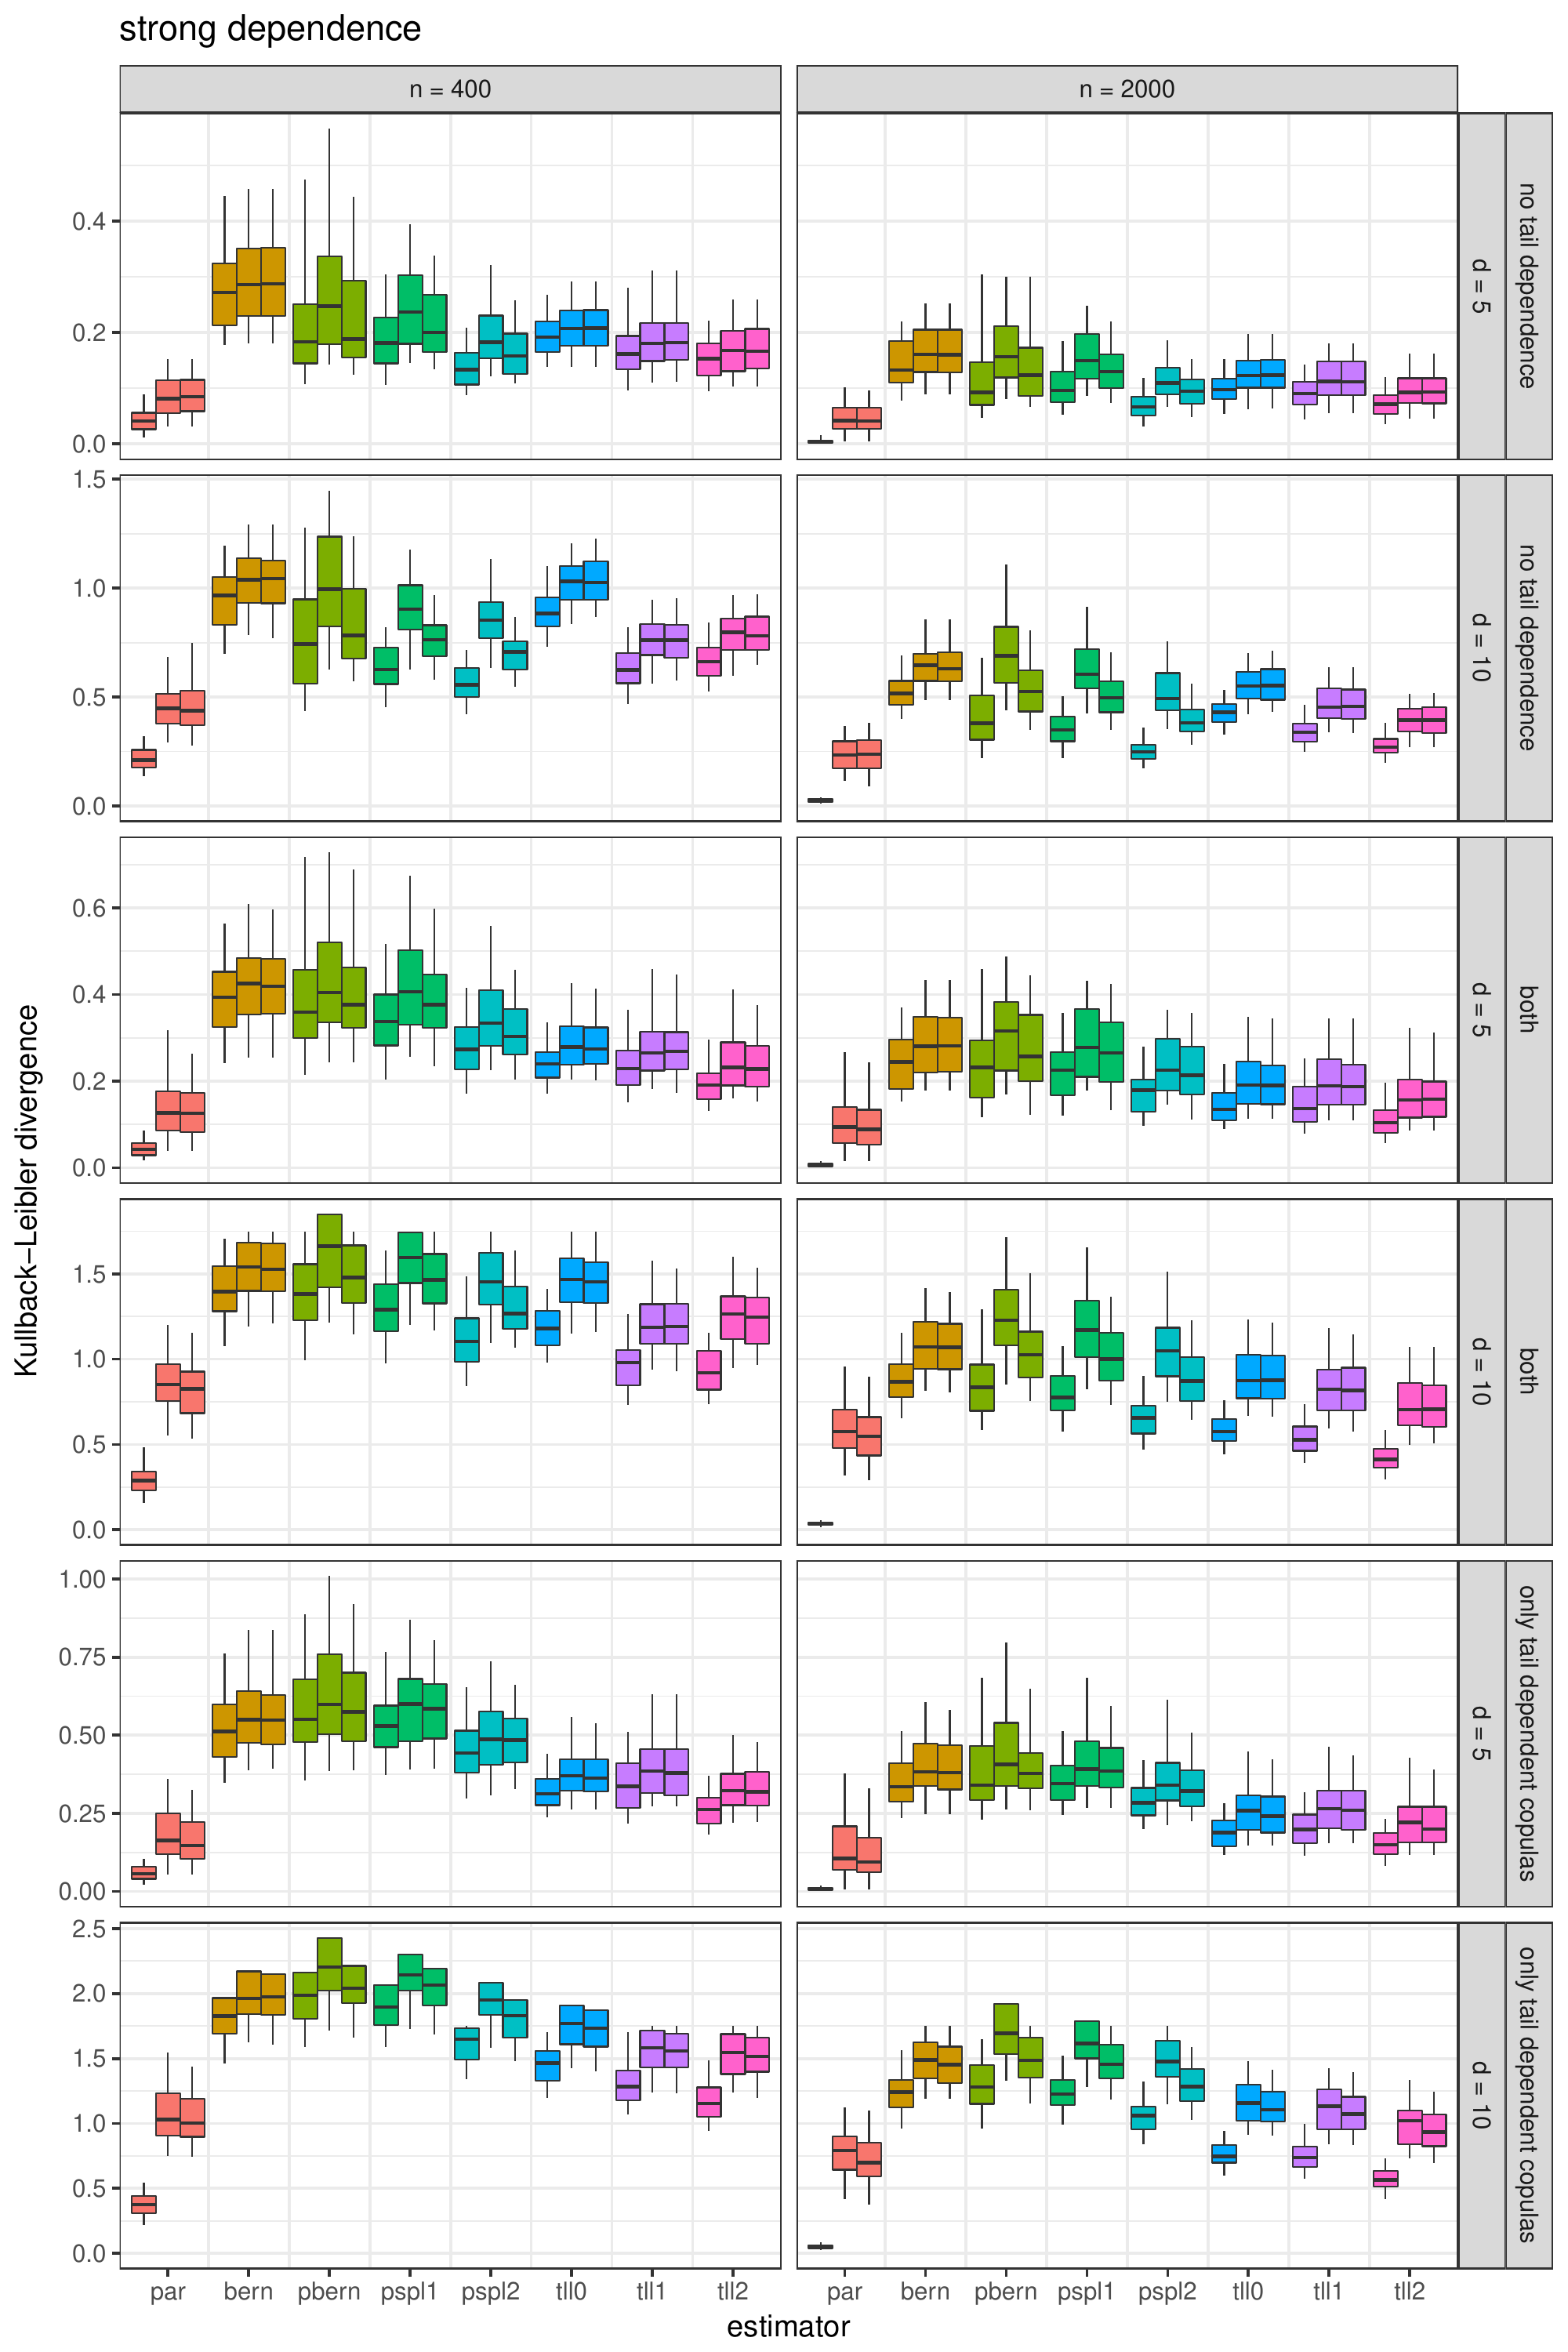} 
\caption{\emph{strong dependence:} the box plots show the Kullback-Leibler divergence achieved by each estimation method. Results are split by sample size, dimension, and type of dependence.  Per estimator there are three boxes, corresponding to estimation under known structure, selection by Kendall's $\tau$, and selection by cAIC (from left to right).}
\end{figure}
